# Supplementary material for: On Data Augmentation for Extreme Multi-label Classification
Source: arXiv:2009.10778 source file (2020-09-22)
Supplement: Supplementary file 1 [file appendix.tex]

\section{Appendices}
\label{sec:appendix}
\subsection{Hyperparameter Settings}
Hyperparameter settings for finetuning GPT-2, ROBERTA and G-DAUG are shown in Table 14, 15, 16, 17 and 18. We manually tune the learn- ing rate and the number of epochs for GPT-2 fine- tuning based on validation perplexity.

\begin{table*}[ht!]\centering
\begin{tabular}{ |c|c|c| c|c|} 
 \hline
 Hyperparameters & RoBERTa (HR)& RoBERTa + LA (HR)  & RoBERTa (HR)& RoBERTa + LA (HR)\\ 
  \hline
 Hardware \\
 \hline
 lr &  1e-6 & 5e-6 & 1e-6 & 1e-6\\ 
\hline
\end{tabular}
\end{table*}
